# Supplementary material for: High-Level Synthesis for Packet-Processing Pipelines
Source: arXiv:2211.06475 source file (2022-11-18)
Supplement: Supplementary file 1 [file appendix.tex]

\section{Proof of Theorem 1}
\label{appendix:contract_gen}
\begin{theorem}
For a given structure, suppose the total number of stages is $2\cdot N$ and the maximum number of tables per stage is w. (w $>$ 2*N). If we know that for one input P4 program, the optimal allocation result uses $m$ stages (m $\leq$ N), it is impossible for one compiler to reject this input program because of table resource constraints as far as this compiler did not leave any stage empty on purpose.
\end{theorem}
\begin{definition}
Let T represent the total number of tables in the given P4 program. Let D represent the depth of the dependency graph among all tables within the input P4 program.
\end{definition}
\begin{proof}
Since the optimal allocation result uses m stages in total, we can draw the conclusion that the T $\leq$ m*w and D $\leq$ m.
Since m $\leq$ N, we can get that T $\leq$ N*w and D $\leq$ N.
We will consider the worst case where T $=$ N*w and D $=$ N.\\
Based on the fact that D $=$ N, we use $n_{i}$ to represent the number of tables in layer i in the dependency graph. One obviously feasible but suboptimal allocation is to allocate tables layer by layer which means the total number of stages should be $\sum_{i=1}^{N}ceil(\frac{n_{i}}{w})$ where ceil(x) represents the integer that is greater than or equal to x. In addition, T $=$ N*w means $\sum_{i=1}^{N}n_{i}=$ N*w. For the worst allocation case, we want to maximize the value of $\sum_{i=1}^{N}ceil(\frac{n_{i}}{w})$\\
We can rewrite $n_{i} = k_{i}*w + \delta_{i}$ where $0 \leq \delta_{i} < w$. If for some i, $\delta_{i} == 0$, ceil($n_{i} / w$) = $k_{i}$. We can find a new $0 < \delta' < w$ and let $n_{i}' = (k_{i} - 1)*w + \delta'$ such that ceil($n_{i}'$) = $k_{i}$. It is easy to prove that $n_{i} > n_{i}'$, which means we use the same number of stages for tables in this layer with more tables left for future stages. Therefore, if we want to maximize the total number of stages, we need to guarantee that for all i, $0 < \delta_{i} < w$.\\
Then, the total number of stages can be written as $\sum_{i=1}^{N}k_{i} + N$. From the constraint $\sum_{i=1}^{N}n_{i}=$ N*w, we can get $(\sum_{i=1}^{N}k_{i})w + \sum_{i=1}^{N}\delta_{i}=$ N*w. If we divide w on both sides, we can get $\sum_{i=1}^{N}k_{i} \leq N$, therefore even the worst case, $\sum_{i=1}^{N}k_{i} + N \leq 2*N$, which can be fit into the structure.
\end{proof}

\section{Proof of Theorem 2}
\label{appendix:benchmark_gen}
\begin{theorem}
For a given structure, suppose the total number of stages is 2*N and the maximum number of tables per stage is w. (w $>$ 2*N). If we know that for one input P4 program, if the optimal allocation result uses N + 1 stages, it is possible for one compiler to reject this input program.
\end{theorem}
\begin{proof}
Generate (w + 1) groups of tables where $table_{i,j + 1}$ is dependent on $table_{i,j}$ for $0 \leq i \leq (w - 1)$ and $0 \leq j \leq (N - 1)$, $table_{w, j + 1}$ is dependent on $table_{w,j}$ for $0 \leq j \leq (N - 1)$.\\
One allocation scenario is to allocate first w groups of table to fill up the first N columns. However, last group which has (N + 1) tables in sequence cannot be placed since there are only N stages remaining.\\
Another allocation scenario is to allocate $table_{w,i}$ for $0 \leq i \leq N$ in the last row. Allocate $table_{w-1,i}$ for $0 \leq i \leq (N - 1)$ diagonally ($table_{w-1,0}$ in the first location of row zero and $table_{w-1,1}$ in the second location of row one etc.) and allocate all tables in the jth group $table_{j,i}$ for $0 \leq i \leq (N - 1)$ in row j. Then, it satisfies all dependency constraints and only use (N + 1) stages.
\end{proof}
